# Supplementary material for: STAR: Scale-wise Text-conditioned AutoRegressive image generation
Source: arXiv:2406.10797 source file (2025-02-19)
Supplement: Supplementary file 1 [file more_ablation.tex]

\section{Additional Ablations}
\subsection{Text Encoders}
Through our framework requires two complementary text representations, a compact embedding $\eta(y)$ for modeling global image structure and a dense embedding $\tau(y)$ for fine-grained textual conditioning. This architectural design enables flexibility in the choice of text encoders. While our primary implementation utilizes the CLIP encoder~\cite{radford2021learning}, empirical evaluations demonstrate the framework's compatibility with alternative encoders, including the T5 text encoder~\cite{raffel2020exploring}.

Specifically, we replace the local representation $\tau(y)$ from CLIP with embedding from pretrained T5-xl encoder. 
Since the training approach of T5 differs from that of CLIP, it lacks the concept of a global token. We retain the global features $\eta(y)$ from CLIP, resulting in a text-guided architecture that combines the two text encoders. As shown in Table~\ref{table_ab_text_rope}, this leads to a performance improvement of XX for the model.

\subsection{Normalization in RoPE}
In~\cref{fig_ab_rope} of main text, we conducted empirical analyses to evaluate our Normalized RoPE design. A critical question emerges: is the normalization step fundamentally necessary, or do the performance improvements stem solely from the advanced RoPE-2D positional embeddings? This ablation study addresses the potential confounding effects between normalization and the underlying positional encoding mechanism.

To illustrate the role of the "normalization" operation in RoPE, we removed the norm operation applied to positional encoding in the main text and applied standard RoPE positional encoding to tokens of different scales. As shown in Table~\ref{table_ab_text_rope}, this resulted in a slight performance drop due to the inconsistency of positional information across tokens of different scales.

\begin{table}[h]
\caption{Ablation of text encoders and positional encodings. Where ``Text" indicates text encoder, specifically, ``CLIP" and ``T5". ``Norm." is short for normalization, refers to the normalization applied in RoPE. Results are acquired with $depth$=16 model under 256 images.}
\label{table_ab_text_rope}
\setlength{\tabcolsep}{2mm}{
\resizebox{0.95\columnwidth}{!}{
\begin{tabular}{ccccc}
\hline
Text & Norm.              & RoPE                       & CLIP-Score$\uparrow$ & FID$\downarrow$ \\ \hline
CLIP & -                          & \ding{55} &     &      \\
CLIP & \ding{55} & \checkmark  &     &      \\
CLIP & \checkmark  & \checkmark  &     &      \\
T5   & \checkmark  & \checkmark  &     &      \\ \hline
\end{tabular}
}}
\end{table}
