# Supplementary material for: STAR: Scale-wise Text-conditioned AutoRegressive image generation
Source: arXiv:2406.10797 source file (2025-02-19)
Supplement: Supplementary file 2 [file ab_text_rope.tex]

\begin{table}[h]
\caption{Ablation of text encoders and positional encodings. Where ``Text" indicates text encoder, specifically, ``CLIP" and ``T5". ``Norm." is short for normalization, refers to the normalization applied in RoPE. Results are acquired with $depth$=16 model under 256 images.}
\label{table_ab_text_rope}
\setlength{\tabcolsep}{2mm}{
\resizebox{0.95\columnwidth}{!}{
\begin{tabular}{ccccc}
\hline
Text & Norm.              & RoPE                       & CLIP-Score$\uparrow$ & FID$\downarrow$ \\ \hline
CLIP & -                          & \ding{55} &     &      \\
CLIP & \ding{55} & \checkmark  &     &      \\
CLIP & \checkmark  & \checkmark  &     &      \\
T5   & \checkmark  & \checkmark  &     &      \\ \hline
\end{tabular}
}}
\end{table}
